# Supplementary material for: DELTACON: A Principled Massive-Graph Similarity Function
Source: arXiv:1304.4657 source file (2013-04-17)
Supplement: Supplementary file 1 [file 100appendix.tex]

TO DO:
\begin{itemize}
\item add a number in abstract
\item explain the state-of-the-art algorithms I used and add citations
\item rephrase the related work
\item add cases of synthetic graphs where \method wins
\item use environment for observations
\item Datasets -- 500 links or 1 to Jure's paper that has links to all of them (o/w, too many references to Jure's papers)?
\item fix caption for synthetic graphs
\item \reminder{we could also run it with heterophily..}
\item VEO instead of EVO (Vertex/Edge Overlap!!!)
\item add more citations in the intro
\item L10 and B10 instead of L5 and B5 - check table with synthetic experimental results
\item FABP or BP should appear only once
\item \checkmark write the intro
\item \checkmark add the conclusions
\end{itemize}

\reminder{ Drop this and the related plot??? 
Another interesting observation springs from the similarity of the graphs to the corresponding empty graph (without edges) which is depicted in Fig. \ref{fig:emptyGraph}. Notice that the fewer the edges in the graph, the greater is its similarity to the empty graph; if we give the ranking of the 5-node graphs starting from the less similar to the more similar graph to the empty one, we have K5 < mK5 < m2K5 < m3K5 < S5 < C5 < P5 < mP5, which totally agrees with our intuition. The same order is maintained for the graphs of 100 nodes, but we observe greater ``gap'' between the similarity scores of the cliques and the ones of the rest graphs since the latter have much fewer edges than the former.
}
